# Supplementary material for: Asymptotic Hodge Theory in String Compactifications and Integrable Systems
Source: arXiv:2409.06794 source file (2024-09-10)
Supplement: Supplementary file 1 [file appendices.tex]

\chapter{Operator relations for Calabi-Yau fourfolds}\label{fourfold_rel}
In the construction of the sl(2)-approximation two operators $\eta$ and $\zeta$ appear, which can be expressed componentwise in terms of $\delta$ with respect to the decomposition \eqref{delta_decomp}. In this appendix we summarize these relations for Calabi-Yau fourfolds. For the purposes of this work we only need $\zeta$, but the expressions for $\eta$ are included for completeness.

Recall that the central identity relating the three operators was given by \eqref{delta-zeta-eta-review}. In the mathematics literature \cite{Kato} this was solved for the components of $\zeta$ for threefolds.\footnote{Furthermore, general expressions for the components $\zeta_{-p,-q}$ and $\eta_{-p,-q}$ in terms of $\delta_{-p,-q}$ were derived, modulo commutators of $\delta_{-r,-s}$ ($r\leq p$ and $s\leq q$) left undetermined.} These results were extended in \cite{Grimm:2021ikg}, where the components of $\eta$ were given in the threefold case. Following the strategy of these works \cite{Kato, Grimm:2021ikg}, we proceed and derive the componentwise expressions for $\eta$ and $\zeta$ for fourfolds. We refer to these articles for a more detailed explanation on how to work out these operator relations. We can express $\zeta$ componentwise in terms of $\delta$ as
\begin{footnotesize}
\begin{align}\label{fourfold_zeta}
 \zeta_{-1,-1}&= \zeta_{-2,-2}= 0\, , \quad \zeta_{-1,-2}= -\frac{i}{2} \delta_{-1,-2}\, , \quad \zeta_{-1,-3} = -\frac{3i}{4} \delta_{-1,-3}\, ,  \quad \zeta_{-1,-4} = -\frac{7i}{8} \delta_{-1,-4}\, ,\nn  \\
\zeta_{-2,-3} &=-\frac{3i}{8} \delta_{-2,-3}+ \frac{1}{8} [\delta_{-1,-2}, \delta_{-1,-1} ]\, , \qquad \zeta_{-2,-4} = -\frac{5i}{8} \delta_{-2,-4} + \frac{1}{4} [ \delta_{-1,-3}, \delta_{-1,-1} ]\, , \nn
\\
 \zeta_{-3,-3} &= \frac{1}{8}[\delta_{-2,-2}, \delta_{-1,-1}]\, ,  \\
\zeta_{-3,-4}  &= -\frac{5i}{16} \delta_{-3,-4} +\frac{3}{16} [\delta_{-2,-3} , \delta_{-1,-1} ] +\frac{3}{16} [\delta_{-1,-3}, \delta_{-2,-1} ] +\frac{i}{48} [\delta_{-1,-1}, [\delta_{-1,-1}, \delta_{-1,-2}]]\, ,  \nn \\
\zeta_{-4,-4} &= \frac{3}{16} [ \delta_{-3,-3}, \delta_{-1,-1} ] +\frac{3}{32} [\delta_{-3,-2} , \delta_{-1,-2}]+\frac{3}{32} [\delta_{-2,-3} , \delta_{-2,-1}]+\frac{i}{32} [\delta_{-1,-1}, [\delta_{-2,-1}, \delta_{-1,-2} ]] \, , \nn
\end{align}
\end{footnotesize}
while $\eta$ is expressed componentwise as
\begin{footnotesize}
\begin{align}\label{fourfold_eta}
\eta_{-1,-1} &= - \delta_{-1,-1}\, , \qquad \eta_{-1,-2} = - \delta_{-1,-2}\, , \qquad \eta_{-1,-3} = - \frac{3}{4}\delta_{-1,-3}\, , \qquad \eta_{-1,-4} = - \frac{1}{2}\delta_{-1,-4}\, , \nn \\
 \eta_{-2,-2} &= - \frac{3}{2} \delta_{-2,-2}\, , \hspace{125.5pt} \eta_{-2,-3} = -\frac{3}{2} \delta_{-2,-3}+\frac{i}{2} [\delta_{-1,-1}, \delta_{-1,-2}]\, , \nn  \\
 \eta_{-2,-4} &= -\frac{5}{4} \delta_{-2,-4}+\frac{5i}{8}[\delta_{-1,-1}, \delta_{-1,-3}]\, , \hspace{30.5pt} \eta_{-3,-3} =  -\frac{15}{8}\delta_{-3,-3}+\frac{5i}{4}[ \delta_{-2,-1}, \delta_{-1,-2}] \, , \nn \\
 \eta_{-3,-4} &= -\frac{15}{8} \delta_{-3,-4}+\frac{3i}{8}[ \delta_{-1,-1},  \delta_{-2,-3}]  \\
 &\quad+\frac{3i}{2}[ \delta_{-2,-1},  \delta_{-1,-3}]+\frac{3i}{4}[ \delta_{-2,-2},  \delta_{-1,-2}] +\frac{1}{8} [  \delta_{-1,-1}, [ \delta_{-1,-1},  \delta_{-1,-2}]]\, , \nn  \\
   \eta_{-4,-4} &= -\frac{35}{16} \delta_{-4,-4} +\frac{63i}{32} [\delta_{-3,-1}, \delta_{-1,-3}]+\frac{21i}{16} [\delta_{-3,-2}, \delta_{-1,-2}]+\frac{21i}{16} [\delta_{-2,-1}, \delta_{-2,-3}] \nn \\
   & \quad +\frac{7}{48}[\delta_{-1,-1},  [\delta_{-1,-1}, \delta_{-2,-2}]]+\frac{7}{24}[\delta_{-2,-1},  [\delta_{-1,-1}, \delta_{-1,-2}]]+\frac{7}{24}[\delta_{-1,-2},  [\delta_{-1,-1}, \delta_{-2,-1}]]\, . \nn
\end{align}
\end{footnotesize}
